# Supplementary material for: PLASTIC: Improving Input and Label Plasticity for Sample Efficient Reinforcement Learning
Source: arXiv:2306.10711 source file (2023-12-08)
Supplement: Supplementary file 1 [file AdditionalExperiments.tex]

\documentclass{article}


% if you need to pass options to natbib, use, e.g.:
%     \PassOptionsToPackage{numbers, compress}{natbib}
% before loading neurips_2023


% ready for submissiit seems that there's not a good complete benchmark for this subfieldon
% \usepackage{neurips_2023}


% to compile a preprint version, e.g., for submission to arXiv, add add the
% [preprint] option:
\usepackage[preprint]{neurips_supp}


% to compile a camera-ready version, add the [final] option, e.g.:
% \usepackage[final]{neurips_2023}


% to avoid loading the natbib package, add option nonatbib:
% \usepackage[nonatbib]{neurips_2023}


\usepackage[utf8]{inputenc} % allow utf-8 input
\usepackage[T1]{fontenc}    % use 8-bit T1 fonts
\usepackage[pagebackref=true, backref=page]{hyperref}       % hyperlinks
\usepackage{url}            % simple URL typesetting
\usepackage{booktabs}       % professional-quality tables
\usepackage{amsfonts}       % blackboard math symbols
\usepackage{nicefrac}       % compact symbols for 1/2, etc.
\usepackage{microtype}      % microtypography
\usepackage{color,xcolor,colortbl}         % colors
\usepackage{multirow}
\usepackage{footnote}
\usepackage{graphicx}
\usepackage{verbatim}
\usepackage{caption}        % subfigure (1)
\usepackage{subcaption}     % subfigure (2)
\usepackage{enumitem}
\usepackage{wrapfig}   % wrap table
\usepackage{multirow}
\usepackage[algo2e, linesnumbered, ruled, vlined ]{algorithm2e}
\usepackage{booktabs} % For better table formatting


\input{math_commands}

% colors and hyperlink setup
\definecolor{darkblue}{rgb}{0.0,0.0,0.65}
\definecolor{darkred}{rgb}{0.65,0.0,0.0}
\definecolor{darkgreen}{rgb}{0.0,0.5,0.0}
\definecolor{tab:blue}{RGB}{31,119,180}  % 1f77b4
\definecolor{tab:red}{RGB}{214,39,40}  % d62728
\definecolor{tab:green}{RGB}{44,160,44}  % 2ca02c
\definecolor{tab:orange}{RGB}{255,127,14}  % ff7f0e
\colorlet{shadecolor}{gray!20}

\hypersetup{
	colorlinks = true,
	citecolor  = darkblue,
	linkcolor  = darkred,
	filecolor  = darkblue,
	urlcolor   = darkgreen,
}


\title{Additional attachment for\\
Enhancing Generalization and Plasticity for \\ Sample Efficient Reinforcement Learning}


% The \author macro works with any number of authors. There are two commands
% used to separate the names and addresses of multiple authors: \And and \AND.
%
% Using \And between authors leaves it to LaTeX to determine where to break the
% lines. Using \AND forces a line break at that point. So, if LaTeX puts 3 of 4
% authors names on the first line, and the last on the second line, try using
% \AND instead of \And before the third author name.

% for comments
\newcommand{\hanseul}[1]{{\color{tab:red}{\bf HS:} #1}}
\newcommand{\daehoon}[1]{\textcolor{blue}{\emph{[DH: #1]}}}


% Convert to regular text
% \renewcommand{\daehoon}[1]{#1}

% Uncomment this to disable comments
% \renewcommand{\daehoon}[1]{}


\author{%
  Hojoon Lee\thanks{Equal contributions.} \quad  Hanseul Cho$^*$ \ \  Hyunseung Kim$^*$ \ \  Daehoon Gwak \ \ Joonkee Kim\\
  {\bfseries  Jaegul Choo\quad Se-Young Yun\quad Chulhee Yun} \\
  Kim Jaechul Graduate School of AI, KAIST \\
  % KAIST AI \\
  \texttt{\{joonleesky, jhs4015, mynsng, daehoon.gwak, joonkeekim,}\\ \texttt{jchoo, yunseyoung, chulhee.yun\}@kaist.ac.kr} \\
}


\begin{document}



\begin{figure}[h]
\begin{center}
\includegraphics[width=0.99\linewidth]{Rebuttal/synthetic_summary (5).pdf}
\end{center}
\vspace{-0.1cm}
\caption{{\bfseries Experiments of baselines on the synthetic experiment.} "B" and "H" denote applying method to the backbone and head of the network respectively. Here, the results are averaged over 30 random seeds with an error bar indicating a 95\% confidence interval. }
\label{figure: abc}
\end{figure}

\vspace{-0.2cm}

\begin{table}[htbp]
\footnotesize
\caption{{\bfseries Exploring various adaptation methods on Atari-100k benchmark.} For L2, we used $\lambda=10^{-4}$ (after tuning). For SAM, we used $\rho=0.1$. The results are averaged over 10 random seeds with reporting 95\% bootstrapped confidence interval.}
\vspace{0.3cm}
\label{tab:my-table}
\centering
\begin{tabular}{cccccccc}
\toprule
 & \multicolumn{6}{c}{Method} &   \\
\cmidrule{2-7}
\multirow{-2}{*}[3pt]{Algorithm} & L2 (B,H) & LN (B) & SAM (B,H) & CReLU (H) & Reset (B,H) & Reset (H) & \multirow{-2}{*}[3pt]{IQM}  \\
\midrule

\multirow{17}{*}{DrQ} &  &  &  &  &  &  & 0.258 (0.224, 0.292)  \\
& \checkmark &  &  &  &  &  & 0.271 (0.227, 0.316) \\
&  & \checkmark &  &  &  &  & 0.259 (0.235, 0.293)  \\
&  & & \checkmark  &  &  &  & 0.325 (0.296, 0.354)  \\
&  &  &  & \checkmark &  &  & 0.256 (0.224, 0.287)  \\
&  &  &  &  & \checkmark &  & 0.132 (0.108, 0.159)  \\
&  &  &  &  &  & \checkmark & \textbf{0.343 (0.314, 0.373)}  \\
\cmidrule{2-8}
%& \checkmark & \checkmark &  &  &  &  & 0.384 (0.335, 0.437) \\
& \checkmark &  &  & \checkmark &  &  & 0.294 (0.252, 0.337) \\
& \checkmark &  &  &  &  & \checkmark & 0.313 (0.280, 0.357) \\
&  & \checkmark  &  & \checkmark &  &  & 0.284 (0.257, 0.314)  \\
&  & \checkmark &  &  &  & \checkmark &  0.396 (0.365, 0.430)  \\
&  &  & \checkmark &  \checkmark &  &  & 0.372 (0.357, 0.408)\\
&  &  & \checkmark &  &  & \checkmark & \textbf{0.411 (0.377, 0.447)} \\
&  &  &  & \checkmark &  & \checkmark & 0.373 (0.344, 0.402)  \\
\cmidrule{2-8}
&  & \checkmark &  & \checkmark &  & \checkmark & 0.433 (0.402, 0.466)  \\
&  & \checkmark & \checkmark & \checkmark &  & \checkmark & \textbf{0.469 (0.433, 0.506)}  \\
\bottomrule
\end{tabular}
\end{table}

\vspace{0.2cm}

% \begin{table}[htbp]
% \footnotesize
% \caption{{\bfseries More RL experiments with DrQ baseline.} For L2, we used $\lambda=10^{-4}$ (after tuning). For SAM, we used $\rho=0.1$.}
% \label{tab:my-table}
% \begin{tabular}{cccccccccc}
% \toprule
%  & \multicolumn{6}{c}{Method} &  &  &  \\
% \cmidrule{2-7}
% \multirow{-2}{*}[3pt]{Algorithm} & SAM & L2(B+H) & LN(B) & Reset(H) & Reset(B) & CReLU(H) & \multirow{-2}{*}[3pt]{IQM} & \multirow{-2}{*}[3pt]{Median} & \multirow{-2}{*}[3pt]{Average} \\
% \midrule
% \multirow{16}{*}{DrQ} & \checkmark &  &  &  &  &  & 0.325 (0.296, 0.354) & 0.327 (0.284, 0.368) & 0.501 (0.465, 0.537) \\
% &  & \checkmark &  &  &  &  & 0.271 (0.227, 0.316) & 0.268 (0.172, 0.358) & 0.558 (0.492, 0.627)\\
% &  &  & \checkmark &  &  &  & 0.259 (0.235, 0.293) & 0.247 (0.218, 0.276) & 0.463 (0.403, 0.522) \\
% &  &  &  & \checkmark &  &  & 0.343 (0.314, 0.373) & 0.291 (0.231, 0.369) & 0.660 (0.611, 0.715) \\
% &  &  &  & \checkmark & \checkmark &  &  &  &  \\
% &  &  &  &  &  & \checkmark & 0.256 (0.224, 0.287) & 0.193 (0.176, 0.252) & 0.498 (0.444, 0.553) \\
% \cmidrule{2-10}
% &  & \checkmark &  &  &  & \checkmark &  &  &  \\
% &  & \checkmark & \checkmark &  &  &  &  &  &  \\
% &  & \checkmark &  & \checkmark &  &  &  &  &  \\
% &  &  &  & \checkmark & \checkmark & \checkmark &  &  &  \\
% &  &  & \checkmark & \checkmark & \checkmark &  &  &  &  \\
% &  &  & \checkmark &  &  & \checkmark & 0.284 (0.257, 0.314) & 0.309 (0.262, 0.332) & 0.476 (0.449, 0.503) \\
% &  &  &  & \checkmark &  & \checkmark & 0.373 (0.344, 0.402) & 0.340 (0.265, 0.385) & 0.708 (0.665, 0.757) \\
% &  &  & \checkmark & \checkmark &  &  & 0.396 (0.365, 0.430) & 0.425 (0.354, 0.471) & 0.702 (0.644, 0.761) \\
% & \checkmark &  &  & \checkmark &  &  & 0.411 (0.377, 0.447) & 0.374 (0.302, 0.458) & 0.753 (0.688, 0.836) \\
% &  &  & \checkmark & \checkmark &  & \checkmark & 0.433 (0.402, 0.466) & 0.475 (0.399, 0.525) & 0.745 (0.709, 0.785) \\
% & \checkmark &  & \checkmark & \checkmark &  & \checkmark & 0.454 (0.416, 0.495) & 0.393 (0.309, 0.523) & 0.890 (0.764, 1.037) \\
% \bottomrule
% \end{tabular}
% \end{table}

\footnotesize
\begin{minipage}[t]{0.5\textwidth}%
          \centering
            \captionof{table}{\textbf{SAM and Reset on Atari-100k with advanced algorithms.} Here, Reset$^\dagger$ indicates the soft reset to the backbone and the hard reset to the head. The results are averaged over 5 random seeds.}
            \label{Tabelle 1}
                \begin{tabular}{cccccc}
                \toprule
                 & \multicolumn{4}{c}{Method} &    \\
                \cmidrule{2-5}
                \multirow{-2}{*}[3pt]{Algorithm} & RR  & SSL & SAM & Reset$^\dagger$ & \multirow{-2}{*}[3pt]{IQM}  \\
                \midrule
                \multirow{6}{*}{SimTPR}
                % & \multirow{3}{*}{2}
                & \multirow{3}{*}{2} 
                   &  &  &                      & 0.366 (0.324, 0.397)    \\
                &  &  &            & \checkmark & 0.709 (0.650, 0.745)    \\
                &  &  & \checkmark & \checkmark & 0.776 (0.703, 0.854)    \\
                \cmidrule{2-6}
                % & \multirow{3}{*}{4}
                & \multirow{3}{*}{4} &  &  &    & 0.243 (0.214, 0.267)    \\
                &  &  &            & \checkmark & 0.780 (0.706, 0.865)    \\
                &  &  & \checkmark & \checkmark & 0.834 (0.769, 0.889)    \\
                \cmidrule{1-6}
                \multirow{4}{*}{BBF} &  
                \multirow{4}{*}{2}
                &  &  & \checkmark  & 0.826 (0.759, 0.895)    \\
                &  & \checkmark &  &  & 0.653 (0.610, 0.698)   \\
                &  & \checkmark &  & \checkmark &  0.940 (0.876, 1.011)   \\
                &  &  & \checkmark & \checkmark &  0.946 (0.833, 1.058)   \\
                
                \bottomrule
                \end{tabular}
\end{minipage} \hspace{0.5cm}
\begin{minipage}[t]{0.38\textwidth}%
            \centering
            \captionof{table}{\textbf{Performance on DMC-GB-500k Benchmark.} The results are averaged over 5 random seeds.}
            \label{Tabelle 2}
                \begin{tabular}{cccc}
                \toprule
                 & \multicolumn{2}{c}{Method} &    \\
                \cmidrule{2-3}
                \multirow{-2}{*}[3pt]{Algorithm} & SAM & Reset & \multirow{-2}{*}[3pt]{IQM}  \\
                \midrule
                \multirow{4}{*}{DrQ} &  &  & 209 (108, 352)     \\
                & \checkmark &  & 270 (168, 397)   \\
                &  & \checkmark & 607 (523, 680)  \\
                & \checkmark & \checkmark & 578 (450, 700) \\
                
                \bottomrule
                \end{tabular}
\end{minipage}%


\end{document}
















% \begin{table}[htbp]
% \footnotesize
% \caption{{\bfseries More RL experiments with DrQ baseline.} For L2, we used $\lambda=10^{-4}$ (after tuning). For SAM, we used $\rho=0.1$.}
% \label{tab:my-table}
% \centering
% \begin{tabular}{ccccccccc}
% \toprule
%  & \multicolumn{6}{c}{Method} &  & \\
% \cmidrule{2-7}
% \multirow{-2}{*}[3pt]{Algorithm} & SAM & L2(B+H) & LN(B) & Reset(H) & Reset(B) & CReLU(H) & \multirow{-2}{*}[3pt]{IQM} & \multirow{-2}{*}[3pt]{Average} \\
% \midrule
% \multirow{16}{*}{DrQ} & \checkmark &  &  &  &  &  & 0.325 (0.296, 0.354) & 0.501 (0.465, 0.537) \\
% &  & \checkmark &  &  &  &  & 0.271 (0.227, 0.316) & 0.558 (0.492, 0.627)\\
% &  &  & \checkmark &  &  &  & 0.259 (0.235, 0.293) & 0.463 (0.403, 0.522) \\
% &  &  &  & \checkmark &  &  & 0.343 (0.314, 0.373) & 0.660 (0.611, 0.715) \\
% &  &  &  & \checkmark & \checkmark &  & 0.132 (0.108, 0.159) & 0.309 (0.271, 0.347) \\
% &  &  &  &  &  & \checkmark & 0.256 (0.224, 0.287) & 0.498 (0.444, 0.553) \\
% \cmidrule{2-9}
% &  & \checkmark & \checkmark &  &  &  &  &  \\
% &  & \checkmark &  & \checkmark &  &  &  &  \\
% &  & \checkmark &  &  &  & \checkmark & 0.294 (0.252, 0.337) & 0.558 (0.485, 0.636) \\
% \cmidrule{2-9}
% &  &  & \checkmark &  &  & \checkmark & 0.284 (0.257, 0.314) & 0.476 (0.449, 0.503) \\
% &  &  &  & \checkmark &  & \checkmark & 0.373 (0.344, 0.402) & 0.708 (0.665, 0.757) \\
% &  &  & \checkmark & \checkmark &  &  & 0.396 (0.365, 0.430) & 0.702 (0.644, 0.761) \\
% & \checkmark &  &  & \checkmark &  &  & 0.411 (0.377, 0.447) & 0.753 (0.688, 0.836) \\
% &  &  & \checkmark & \checkmark &  & \checkmark & 0.433 (0.402, 0.466) & 0.745 (0.709, 0.785) \\
% & \checkmark &  & \checkmark & \checkmark &  & \checkmark & 0.454 (0.416, 0.495) & 0.890 (0.764, 1.037) \\
% \bottomrule
% \end{tabular}
% \end{table}
